# Supplementary material for: Finding a sparse vector in a subspace: Linear sparsity using alternating directions
Source: arXiv:1412.4659 source file (2016-07-20)
Supplement: Supplementary file 1 [file Proof_Main_Theorem.tex]

In this appendix, we prove our main result in Theorem~\ref{thm:recovery}. In particular, we will first show that when the $\mb Y'$ defined in \eqref{eqn:orthonormal-Y'} is the input orthonormal basis, the ``initialization + ADM + LP rounding'' pipeline recovers $\mb x_0$ under the stated technical conditions. Then we will upgrade the recovery result to all orthonormal basis by observing that all three stages are ``invariant'' to the input orthonormal basis $\mb Y$. 

Keep the notation in Section \ref{sec:algorithm}, let $\mb y^1,\cdots,\mb y^p$ be the transpose of the rows of $\mb Y$, and let $\mb y'^1,\cdots,\mb y'^p$ be the transpose of the rows of $\mb Y'$. For $\mb q \in \bb S^{n-1}$, set 
\begin{align}
\mb Q(\mb q) \;&=\; \frac{1}{p}\sum_{k=1}^p \mb y^k S_\lambda \brac{\mb q^\top \mb y^k },\label{eqn:Q_prime}\\
\mb Q'(\mb q) \;&=\; \frac{1}{p} \sum_{k=1}^p \mb y'^k S_\lambda \brac{\mb q^\top \mb y'^k }.
\end{align}
Further, we write $\mb Q\paren{\mb q} = \brac{Q_1\paren{\mb q}; \mb Q_2\paren{\mb q}}$, where $Q_1\paren{\mb q}$ is the first coordinate, and define similar notations for $\mb Q'\paren{\mb q}$. In addition, for any $k=1,\cdots,p$, set 
\begin{align}
X_k^1(Z_k) \;& = \; x_{0k}S_\lambda \brac{\mb q^\top \mb y^k}\; = \; x_{0k} S_\lambda \brac{x_{0k}q_1+Z_k}, \label{X_k_1}\\
\mb X_k^2(Z_k) \; &= \; \mb g^k S_\lambda \brac{\mb q^\top \mb y^k}\; = \; \mb g^k S_\lambda\brac{x_{0k}q_1+Z_k},\label{X_k_2}
\end{align}
where $Z_k = {\bf q}_2^\top \mb g^k \sim \N(0,\sigma^2)$ for $\sigma = \norm{\mb q_2}_2/\sqrt{p}$, and $x_{0k}$ denotes the $k$-th coordinate of $\mb x_0$. Hence we obviously have
\begin{align}
Q_1\; = \; \frac{1}{p}\sum_{k=1}^p X_k^1,\quad \mb Q_2 = \frac{1}{p}\sum_{k=1}^p \mb X_k^2,\label{Q_1_2}.
\end{align}

Next we sketch the main technical pieces for establishing the recovery results for $\mb Y'$ first. All detailed proofs are deferred to later sections of the appendix. We will assume $\frac{1}{2}\exp\paren{n/2} \ge p \ge C n^4 \log n$ for some large constant $C$ for all the subsequent claims. 
\begin{enumerate}
\item \textbf{Good initialization}. Proposition \ref{prop:initialization} in Appendix \ref{app:initialization} shows that with high probability, at least one of our $p$ initialization vectors suggested in Section \ref{sec:algorithm}, say $\mb q_i^{(0)} = \mb y'^i$, obeys that 
\begin{align}
\abs{\innerprod{\frac{\mb y'^i}{\norm{\mb y'^i}_2}}{\mb e_1}} \ge \frac{1}{10\sqrt{\theta n}}.
\end{align}

\item \textbf{Uniform progress away from the equator}. By Proposition \ref{prop:gap-bound-Y'} in Appendix \ref{app:gap-finite}, there exists some constant $\theta_0 > 0$, such that for any $\theta \in \paren{\frac{1}{\sqrt{n}}, \theta_0}$,
\begin{align}
G'(\mb q) = \frac{\abs{Q_1'(\mb q)}}{\abs{q_1}} - \frac{\norm{\mb Q_2'(\mb q)}_2}{\norm{\mb q}_2}\;&\geq \;\frac{1}{10^4\theta^2 np }
\end{align}
holds uniformly for all $\mb q\in \bb S^{n-1}$ in the region $\frac{1}{10\sqrt{\theta n}} \leq \abs{q_1} \leq 3 \sqrt{\theta}$ with high probability.  

\item \textbf{No jumps away from the cap}. Proposition \ref{lem:safe} in Appendix \ref{app:safe-region} shows that for any $\theta \in \paren{\frac{1}{\sqrt{n}}, \theta_0}$, with high probability, 
\begin{align}
\frac{Q_1'(\mb q)}{\norm{\mb Q'(\mb q)}_2}\;\geq \; 2\sqrt{\theta}
\end{align}
holds for all $\mb q$ with $\abs{q_1}\geq 3 \sqrt{\theta}$. 

\item \textbf{Location of the stationary/stopping point}. The first point above ensures that with high probability at least one starting point $\mb q^{\paren{0}}$ will satisfy $\abs{q^{(0)}_1} \ge \frac{1}{10\sqrt{\theta n}}$. As shown in Appendix~\ref{app:iter_cplx}, the strictly positive gap of the second point ensures that one needs to run at most $O\paren{n^4 \log n}$ iterations to first encounter an iterate $\mb q^{(k)}$ such that $\abs{q^{(k)}_1} \ge 3\sqrt{\theta}$. The third point suggests extra iterations will not move away from the cap area, and hence the stationary point $\overline{\mb q}$ of the ADM algorithm will satisfy $\abs{\overline{q}_1} \geq 2\sqrt{\theta}$. If one enforces a hard stop after $O\paren{n^4\log n}$ iterations, the stopping point will similarly stay in the  region $\abs{q_1} \ge 2\sqrt{\theta}$. 

\item \textbf{LP Rounding succeeds}. We know that in the LP rounding stage, described in Section \ref{sec:algorithm}, will receive a vector $\mb r= \bar{\mb q}$ with its first coordinate $|r_1| \geq 2 \sqrt{\theta}$. Proposition \ref{lem:rounding} in Appendix \ref{app:rounding} proves that with high probability, the LP rounding \eqref{eqn:rounding} (operated on $\mb Y'$) will output a solution $\mb q^\star = \mb e_1$. 
\end{enumerate}
In summary, our ADM algorithm in Algorithm \ref{ADM} using a smart initialization, plus an LP rounding stage \eqref{eqn:rounding}, will output $\mb q^\star  = \pm \mb e_1$ with high probability, or $\mb Y'\mb q^\star$ as a nontrivial scaled version of $\mb x_0$. 

For the general case when the input is an arbitrary orthonormal basis $\widehat{\mb Y} = \mb Y' \mb R$ for a certain orthogonal matrix $\mb R$, the target solution is $\mb R^\top \mb e_1$. The following technical pieces are perfectly parallel to the above for $\mb Y'$. 
\begin{itemize}
\item Discussion at the end of Appendix~\ref{app:initialization} suggests with high probability, at least one row of $\widehat{\mb Y}$ provides an initial point $\mb q^{(0)}$ such that $\abs{\innerprod{\mb q^{(0)}}{\mb R^\top \mb e_1}} \ge \frac{1}{10\sqrt{\theta n}}$. 
\item Discussion following Proposition~\ref{prop:gap-bound-Y'} in Appendix~\ref{app:gap-finite} suggests that for all $\mb q$ such that $\frac{1}{10\sqrt{\theta n}} \le \abs{\innerprod{\mb q}{\mb R^\top \mb e_1}} \le 3\sqrt{\theta}$, there is a strictly positive gap, indicating steady progress towards a point $\mb q^{(k)}$ such that $\abs{\innerprod{\mb q^{(k)}}{\mb R^\top \mb e_1}} \ge 3\sqrt{\theta}$. 
\item Discussion at the end of Appendix~\ref{app:safe-region} indicates once $\mb q$ satisfying $\abs{\innerprod{\mb q}{\mb R^\top \mb e_1}}$, the next iterate will not move far away from the target: 
\begin{align}
\frac{\innerprod{\mb Q'\paren{\mb q; \widehat{\mb Y}}}{\mb R^\top \mb e_1}}{\norm{\mb Q'\paren{\mb q; \widehat{\mb Y}}}_2} \ge 2\sqrt{\theta}. 
\end{align}
\item Repeating the argument in Appendix~\ref{app:iter_cplx} for general input $\widehat{\mb Y}$ shows it is enough to run the ADM algorithm $O\paren{n^4 \log n}$ iterations to cross the range $\frac{1}{10\sqrt{\theta n}} \le \abs{\innerprod{\mb q}{\mb R^\top \mb e_1}} \le 3\sqrt{\theta}$. So the above three points together dictates that with the proposed initialization, with high probability, we finally obtain a point $\overline{\mb q}$ that satisfies $\abs{\innerprod{\overline{\mb q}}{\mb R^\top \mb e_1}} \ge 2\sqrt{\theta}$, if we run at least $O\paren{n^4 \log n}$ iterations.  
\item Since the ADM returns $\overline{\mb q}$ satisfying $\abs{\innerprod{\overline{\mb q}}{\mb R^\top \mb e_1}} \ge 2\sqrt{\theta}$, discussion at the end of Appendix~\ref{app:rounding} dictates that we will obtain $\mb q^\star = \mb R^\top \mb e_1$ as the optimizer of the rounding program, exactly the target solution. 
\end{itemize}
We complete the proof.
